# Supplementary material for: Suppression exponent for multiparticle production in $\lambda\phi^{4}$ theory
Source: arXiv:2212.03268 ancillary file (2022-12-06)
Supplement: Supplementary file 1 [file info.pdf]

# Suppression exponent for multiparticle production in $\lambda\phi^4$ theory

## *Ancillary files*

---

S.V. Demidov, B.R. Farkhtdinov, D.G. Levkov

### Notations

Ancillary files 'finite\_J.dat', 'zero\_J.dat', and 'large\_n.dat' provide raw numerical data in text format. Their first two lines start with '#' and briefly summarize file contents. Every next line sequentially lists quantities (floating-point numbers) computed for one semiclassical solution or one extrapolated data point. The quantities within each line are separated by two space characters. The contexts of the files are specified below. We use units with  $m = 1$ .

Ancillary file 'video\_poles.mp4' is a movie demonstrating complex phase of the semiclassical solution  $\phi_{\text{cl}}(t, r)$  by color in complex time plane. The movie frames correspond to sequentially increasing radial coordinate  $r$ . The singularity surfaces  $t_*(r)$ ,  $t'_*(r)$ , etc. of the solution and respective branch cuts are shown by black solid lines and white regions beneath them. The solution parameters and other details are given in Fig. 12b of the main text.

Ancillary files 'solution.mp4' and 'solution\_white.mp4' are movies demonstrating absolute value of complex spherically-symmetric solution  $\phi(t, x, y, z)$  at  $z = 0$  which describes creation of a large number  $n$  of particles from few colliding quanta in the unbroken  $\phi^4$  theory. Color represents complex phase of  $\phi$ . The evolution starts with appearance of a large peak in the center representing the collision. With time, the peak decays into outgoing spherical waves describing produced particles. The solution parameters and other details are given in Fig.5 of the main text.

### **finite\_J.dat**

This file provides quantities computed at fixed energy  $\lambda E$ , multiplicity  $\lambda n$ , and Gaussian source  $J(\mathbf{x}) = j_0 \exp\{-\mathbf{x}^2/2\sigma^2\}$  of strength  $j_0$  and width  $\sigma$ .

It contains 9 columns:

1.  $\varepsilon = (E - mn)/n$ : average kinetic energy of final-state particles;
2.  $j_0/\sigma$ : ratio of the source strength to its width;
3.  $j_0$ : source strength;
4.  $\lambda n/(4\pi)$ : rescaled final-state multiplicity (2.5);
5.  $\lambda \mathcal{E}(t_{N_t+1/2})/(4\pi)$ : rescaled exact energy (2.9) computed at large positive time  $t_{N_t+1/2} = (t_{N_t} + t_{N_t+1})/2$ ;
6.  $\lambda E/(4\pi)$ : rescaled linear final-state energy (2.5);
7.  $T$ : Lagrange multiplier entering Eqs. (2.4) and (2.8);

8.  $\theta$ : Lagrange multiplier entering Eqs. (2.4) and (2.8);
9.  $F_J$ : suppression exponent (2.7) in the case of nonzero source.

### **zero\_J.dat**

This file provides quantities extrapolated to  $j_0 = 0$  at fixed energy  $\lambda E$ , multiplicity  $\lambda n$ , and ratio  $j_0/\sigma$ .

It contains 10 columns:

1.  $\varepsilon = (E - mn)/n$ : average kinetic energy of final-state particles;
2.  $j_0/\sigma$ : ratio of the source strength to its width;
3.  $\lambda n$ : final-state multiplicity (2.5);
4.  $\lambda E$ : linear final-state energy (2.5);
5.  $T$ : Lagrange multiplier entering Eqs. (2.4) and (2.8);
6.  $dT$ : extrapolation error of  $T$ ;
7.  $\theta$ : Lagrange multiplier entering Eqs. (2.4) and (2.8);
8.  $d\theta$ : extrapolation error of  $\theta$ ;
9.  $F$ : suppression exponent (1.5) at  $J = 0$ ;
10.  $dF$ : extrapolation error of  $F$ .

### **large\_n.dat**

This file provides the slope  $f_\infty(\varepsilon)$  and shift  $g_\infty(\varepsilon)$  of the suppression exponent at  $\lambda n \rightarrow +\infty$ , see Eq. (1.6). The data are obtained by fitting the numerical values of  $F(\lambda n, \varepsilon)$  with Eq. (4.5). For convenience, we also provide function  $f(\varepsilon)$  entering the tree-level expression (4.4) for the suppression exponent. This latter function is computed using the method of Ref. [62].

This file contains 6 columns:

1.  $\varepsilon = (E - mn)/n$ : average kinetic energy of final-state particles;
2.  $f_\infty(\varepsilon)$ : slope of the suppression exponent at large  $\lambda n$ , see Eq. (1.6);
3.  $df_\infty$ : extrapolation error of  $f_\infty(\varepsilon)$ ;
4.  $g_\infty(\varepsilon)$ : shift of suppression exponent at large  $\lambda n$ , see Eq. (1.6);
5.  $dg_\infty$ : extrapolation error of  $g_\infty(\varepsilon)$ ;
6.  $f(\varepsilon)$ : function entering the tree-level expression for  $F$ , see Eq. (4.4).
